# Supplementary material for: Types by Need (Extended Version)
Source: arXiv:1902.05945 source file (2019-02-15)
Supplement: Supplementary file 1 [file toappendix.tex]

\gettoappendix {prop:syntactic-characterization-closed-normal}
\gettoappendix {l:name-linear-substitution}
\gettoappendix {prop:name-subject-reduction}
\gettoappendix {prop:name-normal-forms-forall}
\gettoappendix {thm:name-correctness}
\gettoappendix {prop:name-normal-forms-exist}
\gettoappendix {l:name-linear-removal}
\gettoappendix {prop:name-subject-expansion}
\gettoappendix {thm:name-completeness}
\gettoappendix {l:value-linear-substitution-bis}
\gettoappendix {prop:value-subject-reduction}
\gettoappendix {prop:value-normal-forms-forall}
\gettoappendix {thm:value-correctness}
\gettoappendix {prop:value-normal-forms-exist}
\gettoappendix {l:value-linear-anti-substitution}
\gettoappendix {prop:value-subject-expansion}
\gettoappendix {thm:value-completeness}
\gettoappendix {l:need-linear-substitution}
\gettoappendix {prop:need-subject-reduction}
\gettoappendix {prop:need-normal-forms-forall}
\gettoappendix {thm:need-correctness}
\gettoappendix {prop:need-normal-forms-exist}
\gettoappendix {l:need-linear-anti-substitution}
\gettoappendix {prop:need-subject-expansion}
\gettoappendix {thm:need-completeness}
\gettoappendix {coro:value-need}
\gettoappendix {cor:value-longer-than-need}
